# Supplementary material for: Incommensurate phonon anomaly and the nature of charge density waves in cuprates
Source: arXiv:1712.04554 ancillary file (2017-12-15)
Supplement: Supplementary file 1 [file Supplementary.pdf]

# Supplementary Materials for Incommensurate phonon anomaly and the nature of charge density waves in cuprates

H. Miao,<sup>1,\*</sup> D. Ishikawa,<sup>2,3</sup> R. Heid,<sup>4</sup> M. Le Tacon,<sup>4</sup> G. Fabbri,<sup>1</sup>  
D. Meyers,<sup>1</sup> G. D. Gu,<sup>1</sup> A. Q. R. Baron,<sup>2</sup> and M. P. M. Dean<sup>1,†</sup>

<sup>1</sup>Condensed Matter Physics and Materials Science Department,  
Brookhaven National Laboratory, Upton, New York 11973, USA

<sup>2</sup>Materials Dynamics Laboratory, RIKEN SPring-8 Center, RIKEN, Sayo, Hyogo, Japan

<sup>3</sup>Research and Utilization Division, SPring-8/JASRI, Sayo, Hyogo, Japan

<sup>4</sup>Institut für Festkörperphysik, Karlsruher Institut für Technologie, P.O. Box 3640, D-76021 Karlsruhe, Germany  
(Dated: December 15, 2017)

## I. FIRST PRINCIPLES PHONON CALCULATIONS

The phonon dynamic structure factor weighted by the x-ray atomic form factors was calculated using density functional perturbation theory (DFPT). Since the mass of the La and Ba atoms are similar, calculations were performed using  $\text{La}_2\text{CuO}_4$  without accounting for the doping. We used the low-temperature tetragonal (LTT) structure as a starting point and relaxed the atomic positions in order to minimize the energy. We use a pseudopotential method with a special variant of the basis set (so-called mixed basis), which can deal rather efficiently with transition metal compounds [1]. Norm-conserving pseudopotentials including partial core corrections are constructed following the scheme of Vanderbilt [2]. 3s and 3p semi-core states of Cu and 5p and 5d semi-core states of La are treated as valence states. La f states are not taken into account explicitly. The basis sets consist of local functions of s, p and d symmetry at the Cu and La sites, and of s and p symmetry at the O sites, augmented with plane waves up to a cutoff energy of 24 Ry. The exchange-correlation functional is treated in the local-density approximation (LDA) using the form given by Perdew and Wang [3]. Under such approximations, the electronic ground state is metallic (as opposed to the real material  $\text{La}_2\text{CuO}_4$ , which is known to be a Mott insulator), which actually better represents the hole doped case. Brillouin zone summations are carried out with tetragonal  $8 \times 8 \times 4$   $k$ -point meshes in combination with a Gaussian broadening of 0.2 eV. Dynamical matrices on a  $2 \times 2 \times 2$  mesh of phonon momenta are calculated with DFPT as implemented in the mixed-basis pseudopotential method [4]. Dynamical matrices at arbitrary  $\mathbf{Q}$  are then obtained by standard Fourier interpolation, and  $S(\mathbf{Q}, \omega)$  is derived from the related phonon frequencies and eigenvectors. As shown in Fig. 1, these calculations reproduce the measured phonon energies at  $\mathbf{Q}$ -vectors away from the CDW within the expected accuracy of a couple of meV and justifies the phonon fitting procedure.

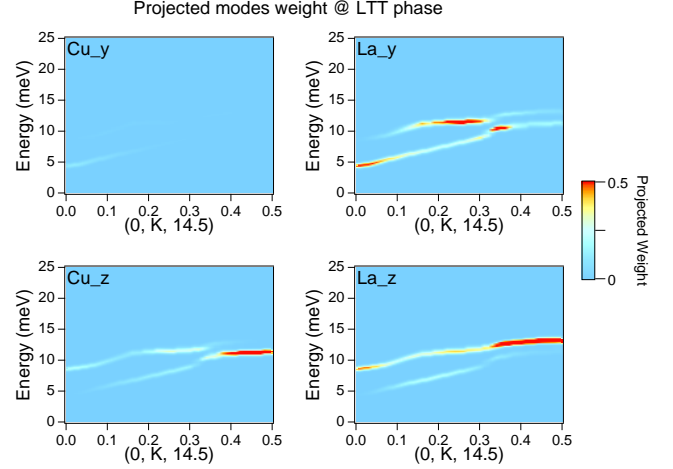

Figure 1. Projected Cu-y, Cu-z, La-y and La-z atomic motions on M1 and M2 modes.

This also clarifies that the overall effect of the CDW on the phonons in general is rather small, which is expected as only a relatively small fraction of the electrons participate in the CDW. Strong effects are localized in a small range reciprocal space around the CDW wavevector.

Our DFPT calculation shows that the M1 and M2 modes are associated with z and y direction motions of the heavier La and Cu atoms. Figure 1 shows the projected Cu and La motions on M1 and M2 modes. We find that besides the Cu-y motion, all other atomic motions are mixed in M1 and M2 and showing a strong momentum dependence, which is expected considering the experimental data is collected away from high crystal symmetry lines. Therefore neither M1 nor M2 can be assigned to a purely longitudinal or transverse mode. The calculation finds that M1 has primarily transverse acoustic character and M2 has mixed longitudinal acoustic and longitudinal optical character. These modes connect to the transverse and longitudinal branches of the  $[0,0,L]$  direction, respectively.

In an electron-phonon coupling driven CDW scenario we note that one expects the phonon modes to soften to zero (or very low) energy at the transition. Furthermore, below the transition one might expect new modes related to the CDW to exist dispersing out of a CDW Bragg

\* hmiao@bnl.gov

† mdean@bnl.gov

peak. In our measurement, we see only partial phonon softening, so we do not expect to be able to see such modes. Furthermore the structure factor of such modes could be far weaker than those studied here.

## II. FITTING OF PHONON SPECTRA

The data were fit using a sum of the signals from different phonon modes, multiplied by the Bose factor and convoluted with the energy resolution function  $R(\omega)$  (Eq. B1 of the main text). We also include an intensity-scaled resolution function to represent the elastic line  $R_{\text{el}}$  and a constant offset  $I_c$ , such that

$$S(\mathbf{Q}, \omega) = \sum_i \frac{\chi_i''(\mathbf{Q}, \omega)}{1 - e^{-\omega/k_B T}} * R(\omega) + R_{\text{el}}(\omega) + I_c. \quad (1)$$

Here phonon modes are represented by the damped harmonic oscillator form [5]

$$\chi_i''(\mathbf{Q}, \omega) = \frac{4A_i\gamma_i\omega\omega_i}{\pi[(\omega^2 - \omega_i^2)^2 + 4\omega^2\gamma_i^2]} \quad (2)$$

where  $A_i$ ,  $\omega_i$  and  $2\gamma_i$  are the intensity, energy and full width at half maximum of phonon peak  $i$  at the measured wavevector,  $\mathbf{Q}$ . The exact form of the resolution function for each analyzer in the slit setting used for the experiment was determined by fitting the elastic line at low temperature. At each momentum transfer, the number of phonon peaks at different temperatures is fixed. Although the development of uniform long-range CDW order would be expected to cause splitting and folding effects on the phonon spectra, as we discussed in the main text, the CDW correlation, even in the ordered phase, is dominated ( $\sim 90\%$  [6]) by very short correlation length fluctuations. On this basis, possible folding and splitting effects would be expected to be weak. We carefully examined the lineshapes of the observed peaks and found that they are well-described within a scheme where the number of modes is fixed by the DFPT predictions, so we used this approach in the data analysis. Indeed, as we show in Fig. 2 of the main text, the phonon spectra away from  $\mathbf{Q}_{\text{CDW}}$  do not change across the CDW transition temperature, while the phonon spectra near  $\mathbf{Q}_{\text{CDW}}$  become narrower. This low temperature phonon narrowing is opposite to what is expected in the presence of phonon-splitting supporting our approach.

Non-linear least squares minimization as implemented in Ref. [7] was used to fit the model to the data. Error-bars on fitted parameters are the standard error from the diagonal elements of the covariance matrix. We further confirmed the robustness of small effects such as the reduced width of M2 at  $K = 0.24$  r.l.u. for 12 and 45 K by computing the confidence interval which tests for, and was able to exclude, possible problems due to correlated fitting parameters.

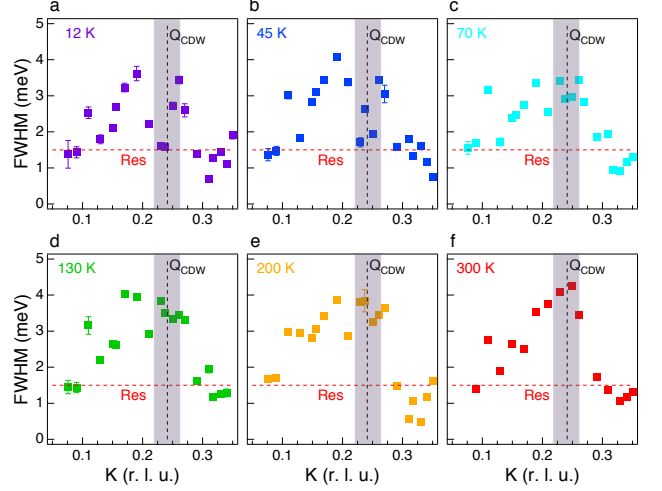

Figure 2. (a)-(f) Momentum dependent M2 phonon scattering rate at 12, 45, 70, 130, 200 and 300 K respectively. The vertical and horizontal dashed lines represent  $\mathbf{Q}_{\text{CDW}}$  and the instrumental energy resolution, respectively. The purple shaded area represent the width of the CDW peak shown in Fig. 4 of the main text.

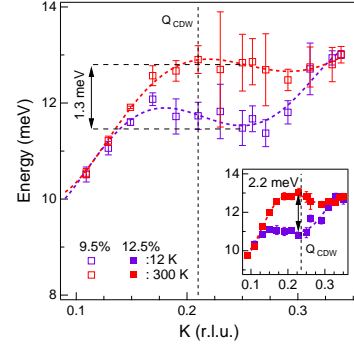

Figure 3. Doping dependence of the phonon anomaly in  $\text{La}_{2-x}\text{Ba}_x\text{CuO}_4$ . The M2 phonon dispersion of  $x = 0.095$  is plotted with open symbols and compared to results for  $x = 0.125$  in the inset. Colored dashed lines are guides to the eyes and vertical black dotted lines mark the CDW ordering wavevector [8].  $x = 0.095$  has a weaker phonon anomaly than  $x = 0.125$  as indicated by the arrow.

## III. MOMENTUM DEPENDENT PHONON SCATTERING RATE

The momentum dependent M2 phonon widths measured at all temperatures are shown in Fig. 2. The sudden drop of the scattering rate is confined to a narrow range near  $\mathbf{Q}_{\text{CDW}}$  and only observed below  $T_{\text{CDW}} = 54$  K. The gray shaded area represents the width of the ordered-CDW peak at 23 K shown in Fig. 4 of the main text. The vertical and horizontal dashed lines represent  $\mathbf{Q}_{\text{CDW}}$  and the instrumental energy resolution, respectively.

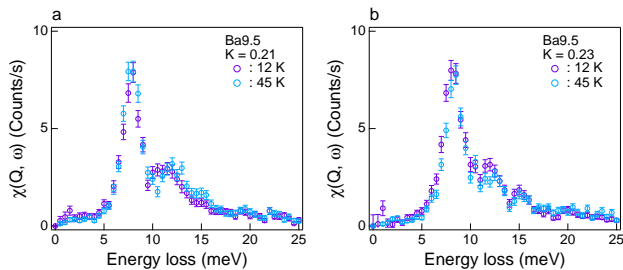

Figure 4. (a) and (b) Elastic line subtracted and Bose-factor corrected IXS spectra of  $\text{La}_{1.905}\text{Ba}_{0.095}\text{CuO}_4$  at  $K = 0.21$  and  $0.23$  r.l.u. respectively. Purple and cyan curve are data below (12 K) and above (45 K) the superconducting transition temperature at 31 K.

#### IV. DOPING DEPENDENCE OF THE PRECURSOR PHONON ANOMALY

To further investigate the nature of the phonon anomalies, we performed the same measurement on more underdoped  $\text{La}_{1.905}\text{Ba}_{0.095}\text{CuO}_4$ . The cooling-induced softening observed in Fig. 3 is significantly weaker 1.3(4) meV in  $x = 0.095$  compared to 2.2(2) meV in  $x = 0.125$  con-

firmed that these effects are due to CDW correlations, which are expected to be weaker away from  $x = 0.125$  [8]. No changes in phonon energy or width are detected through the superconducting transition at 31 K (Supp. IV). We find that in  $x = 0.095$ , the maximum softening occurs at larger wavevectors than the CDW ordering wavevector of 0.21 [8] and that the inflection points in the dispersion occur at similar locations to  $x = 0.125$  (0.24 at 12 K and 0.3 at 300 K). This is again consistent with the weakly doping dependent CDW wavevector in  $\text{YBa}_2\text{Cu}_3\text{O}_{6+\delta}$  supporting our previous interpretations [9, 10].

#### V. THE EFFECT OF SUPERCONDUCTIVITY

Since previous phonon measurements in  $\text{YBa}_2\text{Cu}_3\text{O}_{6+\delta}$ , detected changes in the phonon spectra upon cooling through the superconducting transition temperature  $T_c$  [11], we checked for similar effects in  $\text{La}_{1.905}\text{Ba}_{0.095}\text{CuO}_4$ . Figure 4 shows the IXS spectra below and above  $T_c$  at  $K = 0.21$  and  $0.23$  r.l.u. We do not detect any statistically significant changes and estimate that phonon softening effects, if present, are smaller than 0.5 meV.

- 
- [1] B. Meyer, C. Elsässer, and M. Fähnle, “Fortran90 program for mixed-basis pseudopotential calculations for crystals,” Max-Planck-Institut für Metallforschung, Stuttgart (Unpublished).
  - [2] D. Vanderbilt, “Optimally smooth norm-conserving pseudopotentials,” *Phys. Rev. B* **32**, 8412–8415 (1985).
  - [3] J. P. Perdew and Y. Wang, “Accurate and simple analytic representation of the electron-gas correlation energy,” *Phys. Rev. B* **45**, 13244–13249 (1992).
  - [4] R. Heid and K.-P. Bohnen, “Linear response in a density-functional mixed-basis approach,” *Phys. Rev. B* **60**, R3709–R3712 (1999).
  - [5] B. Fåk and B. Dorner, “Phonon line shapes and excitation energies,” *Physica B: Condensed Matter* **234**, 1107 – 1108 (1997).
  - [6] H. Miao, J. Lorenzana, G. Seibold, Y. Y. Peng, A. Amorese, F. Yakhov-Harris, K. Kummer, N. B. Brookes, R. M. Konik, V. Thampy, G. D. Gu, G. G. Ghiringhelli, L. Braicovich, and M. P. M. Dean, “Precursor charge density waves in  $\text{La}_{1.875}\text{Ba}_{0.125}\text{CuO}_4$ ,” *arXiv* (2017), arXiv:1701.00022.
  - [7] M. Newville, T. Stensitzki, D. B. Allen, and A. Ingargiola, “LMFIT: Non-Linear Least-Square Minimization and Curve-Fitting for Python,” (2014).
  - [8] M. Hücker, M. v. Zimmermann, G. D. Gu, Z. J. Xu, J. S. Wen, Guangyong Xu, H. J. Kang, A. Zheludev, and J. M. Tranquada, “Stripe order in superconducting  $\text{La}_{2-x}\text{Ba}_x\text{CuO}_4$  ( $0.095 \leq x \leq 0.155$ ),” *Phys. Rev. B* **83**, 104506 (2011).
  - [9] G. Ghiringhelli, M. Le Tacon, M. Minola, S. Blanco-Canosa, C. Mazzoli, N. B. Brookes, G. M. De Luca, A. Frano, D. G. Hawthorn, F. He, T. Loew, M. Moretti Sala, D. C. Peets, M. Salluzzo, E. Schierle, R. Sutarto, G. A. Sawatzky, E. Weschke, B. Keimer, L. Braicovich, M. Le Tacon, M. Minola, S. Blanco-Canosa, C. Mazzoli, N. B. Brookes, G. M. De Luca, A. Frano, D. G. Hawthorn, F. He, T. Loew, M. Moretti Sala, D. C. Peets, M. Salluzzo, E. Schierle, R. Sutarto, G. A. Sawatzky, E. Weschke, B. Keimer, and L. Braicovich, “Long-Range Incommensurate Charge Fluctuations in  $(\text{Y,Nd})\text{Ba}_2\text{Cu}_3\text{O}_{6+x}$ ,” *Science* **337**, 821–825 (2012).
  - [10] R. Comin and A. Damascelli, “Resonant X-Ray Scattering Studies of Charge Order in Cuprates,” *Annual Review of Condensed Matter Physics* **7**, 369–405 (2016).
  - [11] M. Le Tacon, A. Bosak, S. M. Souliou, G. Dellea, T. Loew, R. Heid, K.-P. Bohnen, G. Ghiringhelli, M. Krisch, and B. Keimer, “Inelastic X-ray scattering in  $\text{YBa}_2\text{Cu}_3\text{O}_{6.6}$  reveals giant phonon anomalies and elastic central peak due to charge-density-wave formation,” *Nat Phys* **10**, 52–58 (2014).
